# Supplementary material for: Self-prediction residuals improve single-pass detection of wrong-object boxes in grounded vision-language models
Source: arXiv:2611.28632 source file (2026-11-21)
Supplement: Supplementary file 2 [file xlabels-supp.tex]

\newlabel{sec:intro}{{1}{2}{}{}{}}
\newlabel{sec:intro@cref}{{[section][1][]1}{[1][1][]2}{}{}{}}
\newlabel{tab:position}{{1}{4}{}{}{}}
\newlabel{tab:position@cref}{{[table][1][]1}{[1][3][]4}{}{}{}}
\newlabel{sec:related}{{2}{5}{}{}{}}
\newlabel{sec:related@cref}{{[section][2][]2}{[1][5][]5}{}{}{}}
\newlabel{sec:method}{{3}{8}{}{}{}}
\newlabel{sec:method@cref}{{[section][3][]3}{[1][8][]8}{}{}{}}
\newlabel{sec:method:setup}{{3.1}{8}{}{}{}}
\newlabel{sec:method:setup@cref}{{[subsection][1][3]3.1}{[1][8][]8}{}{}{}}
\newlabel{fig:method}{{1}{9}{}{}{}}
\newlabel{fig:method@cref}{{[figure][1][]1}{[1][9][]9}{}{}{}}
\newlabel{sec:method:residual}{{3.2}{9}{}{}{}}
\newlabel{sec:method:residual@cref}{{[subsection][2][3]3.2}{[1][9][]9}{}{}{}}
\newlabel{eq:readout}{{1}{9}{}{}{}}
\newlabel{eq:readout@cref}{{[equation][1][]1}{[1][9][]9}{}{}{}}
\newlabel{eq:residual}{{2}{9}{}{}{}}
\newlabel{eq:residual@cref}{{[equation][2][]2}{[1][9][]9}{}{}{}}
\newlabel{sec:method:design}{{3.3}{10}{}{}{}}
\newlabel{sec:method:design@cref}{{[subsection][3][3]3.3}{[1][10][]10}{}{}{}}
\newlabel{sec:method:combine}{{3.4}{10}{}{}{}}
\newlabel{sec:method:combine@cref}{{[subsection][4][3]3.4}{[1][10][]10}{}{}{}}
\newlabel{eq:combine}{{3}{11}{}{}{}}
\newlabel{eq:combine@cref}{{[equation][3][]3}{[1][10][]11}{}{}{}}
\newlabel{sec:method:probe}{{3.5}{11}{}{}{}}
\newlabel{sec:method:probe@cref}{{[subsection][5][3]3.5}{[1][11][]11}{}{}{}}
\newlabel{alg:detector}{{1}{12}{}{}{}}
\newlabel{alg:detector@cref}{{[algorithm][1][]1}{[1][11][]12}{}{}{}}
\newlabel{sec:method:use}{{3.6}{12}{}{}{}}
\newlabel{sec:method:use@cref}{{[subsection][6][3]3.6}{[1][11][]12}{}{}{}}
\newlabel{sec:setup}{{4}{13}{}{}{}}
\newlabel{sec:setup@cref}{{[section][4][]4}{[1][13][]13}{}{}{}}
\newlabel{tab:lists}{{2}{14}{}{}{}}
\newlabel{tab:lists@cref}{{[table][2][]2}{[1][13][]14}{}{}{}}
\newlabel{sec:plug}{{5}{16}{}{}{}}
\newlabel{sec:plug@cref}{{[section][5][]5}{[1][15][]16}{}{}{}}
\newlabel{sec:plug:add}{{5.1}{16}{}{}{}}
\newlabel{sec:plug:add@cref}{{[subsection][1][5]5.1}{[1][15][]16}{}{}{}}
\newlabel{fig:plugin}{{2}{18}{}{}{}}
\newlabel{fig:plugin@cref}{{[figure][2][]2}{[1][17][]18}{}{}{}}
\newlabel{tab:plugingain}{{3}{18}{}{}{}}
\newlabel{tab:plugingain@cref}{{[table][3][]3}{[1][17][]18}{}{}{}}
\newlabel{sec:plug:detector}{{5.2}{18}{}{}{}}
\newlabel{sec:plug:detector@cref}{{[subsection][2][5]5.2}{[1][17][]18}{}{}{}}
\newlabel{tab:spredrep}{{4}{20}{}{}{}}
\newlabel{tab:spredrep@cref}{{[table][4][]4}{[1][19][]20}{}{}{}}
\newlabel{sec:plug:offideal}{{5.3}{20}{}{}{}}
\newlabel{sec:plug:offideal@cref}{{[subsection][3][5]5.3}{[1][19][]20}{}{}{}}
\newlabel{tab:ablationmain}{{5}{21}{}{}{}}
\newlabel{tab:ablationmain@cref}{{[table][5][]5}{[1][19][]21}{}{}{}}
\newlabel{sec:measure}{{6}{21}{}{}{}}
\newlabel{sec:measure@cref}{{[section][6][]6}{[1][21][]21}{}{}{}}
\newlabel{sec:measure:own}{{6.1}{21}{}{}{}}
\newlabel{sec:measure:own@cref}{{[subsection][1][6]6.1}{[1][21][]21}{}{}{}}
\newlabel{fig:second}{{3}{22}{}{}{}}
\newlabel{fig:second@cref}{{[figure][3][]3}{[1][22][]22}{}{}{}}
\newlabel{sec:measure:second}{{6.2}{22}{}{}{}}
\newlabel{sec:measure:second@cref}{{[subsection][2][6]6.2}{[1][21][]22}{}{}{}}
\newlabel{sec:measure:pull}{{6.3}{22}{}{}{}}
\newlabel{sec:measure:pull@cref}{{[subsection][3][6]6.3}{[1][22][]22}{}{}{}}
\newlabel{fig:pull}{{4}{23}{}{}{}}
\newlabel{fig:pull@cref}{{[figure][4][]4}{[1][23][]23}{}{}{}}
\newlabel{fig:examples}{{5}{24}{}{}{}}
\newlabel{fig:examples@cref}{{[figure][5][]5}{[1][23][]24}{}{}{}}
\newlabel{sec:measure:not}{{6.4}{24}{}{}{}}
\newlabel{sec:measure:not@cref}{{[subsection][4][6]6.4}{[1][23][]24}{}{}{}}
\newlabel{sec:discussion}{{7}{24}{}{}{}}
\newlabel{sec:discussion@cref}{{[section][7][]7}{[1][24][]24}{}{}{}}
\newlabel{sec:limits}{{7}{26}{}{}{}}
\newlabel{sec:limits@cref}{{[section][7][]7}{[1][26][]26}{}{}{}}
\newlabel{sec:conclusion}{{8}{26}{}{}{}}
\newlabel{sec:conclusion@cref}{{[section][8][]8}{[1][26][]26}{}{}{}}
